# Supplementary material for: D{\epsilon}pS: Delayed {\epsilon}-Shrinking for Faster Once-For-All Training
Source: arXiv:2407.06167 source file (2024-07-08)
Supplement: Supplementary file 1 [file 07_appendix.tex]

\section{Appendix A: Code Release}
We make the code of \proposedTraining available at - 

\href{https://anonymous.4open.science/r/des-6F54/}{https://anonymous.4open.science/r/des-6F54/}. The code includes instructions to setup, and run the experiments reported in the paper. 

\section{Appendix B: IKD Warmup}
In this section, we provide evidence of the usefulness of IKD Warmup proposed in \proposedTraining. When distilling knowledge from teacher (full model) to student (smaller subnets) it is important to ensure that the student subnets are not being overly biased to the full model. On the other hand, we need the teacher to provide valuable knowledge to the student subnets. The sweet spot is for the teacher to provide valuable knowledge to the student subnets without completely biasing them. We compute class correlation heatmaps of a partially trained and completely trained full model and visualize them below. 

\textbf{Heatmap calculation.} Average logits for each class are computed by filtering out predictions of each class (denote by $C_i$). For each class, cosine similarity is computed with all other classes to generate the heatmap. Element $A_{ij}$ in the heatmap is the cosine similarity of average logits $C_i$ and $C_j$.

Figure \ref{fig:supp:1k} depicts the class correlation heatmaps of the partially trained and completedly trained full model on ImageNet-1k. The partially trained full model has richer information about non-target classes.

\begin{figure}[ht]
\centering
\begin{subfigure}[ht]{\columnwidth}
     \includegraphics[width=\columnwidth]{supp/1k.pdf}
     \label{fig:supp:1k_sf}
\end{subfigure}
\caption{\small Heatmaps of the class correlation scores for the partially trained and completely trained full model on the ImageNet-1k dataset. Brighter colors imply more diversity in the model.}
\label{fig:supp:1k}
\end{figure}

Figure \ref{fig:supp:200} shows a zoomed version of \ref{fig:supp:1k} focusing on the first 200 classes of the ImageNet-1k dataset
\begin{figure}[h]
\centering
\begin{subfigure}[ht]{\columnwidth}
     \includegraphics[width=\columnwidth]{supp/200.pdf}
     \label{fig:supp:200_sf}
\end{subfigure}
\caption{\small Class correlation heatmaps of the first 200 classes on ImageNet-1k. Brighter colors imply more diversity in the model.}
\label{fig:supp:200}
\end{figure}

\newpage
\section{Appendix C: Training Details}
In this section, we present details of the training hyperparameters used for all our experiments. Unless explicitly specified, we use SGD with nesterov momentum (0.9) and a CosineAnnealingLR schedule for \proposedTraining and BigNAS. To improve generalization, we use label smoothing (0.1) and AutoAugment for all experiments. Post training, we report each subnet's performance after calibrating all batch norm layers on a subset of the training data.

All methods are evaluated on the \textbf{same} DNN architecture search space to isolate the impact of the supernet training algorithm. This is a key difference between BigNAS's experimental setup and ours. BigNAS \cite{bignas} trains models in the 200M to 2000M FLOPs range with the largest network being 4x FLOPs than the largest network in our MobileNetV3 DNN architecture search space.

To train a supernet in \proposedTraining and BigNAS, 4 subnets are sampled per minibatch of data (smallest subnet, largest subnet and 2x randomly sampled subnets). This sampling strategy is called sandwich sampling \cite{universallyslimmable}. On all experiments with BigNAS, we use a LR schedule with constant ending at 5\% of initial learning rate, batch-norm initialization, inplace distillation. Regularization is applied only to the largest network. 

\subsection{ImageNet-1k}
\proposedTraining is trained for 270 epochs with a full warmup period of 150 epochs (\fullModelWarmupSym=55\%). We use an initial learning rate of 0.1625 per batch size 128. The total effective batch size is 2048 split across 16 A40 GPUs. For regularization, weight decay (3e-5) and dropout (p=0.1) are used. We train OFA as is without any changes to hyperparameters. To train BigNAS on the MobileNetV3 based DNN architecture space, we use the hyperparameters as described in the paper. We use RMSProp with a constant learning rate ending at 5\%. The key difference is the DNN architecture search space i.e. MobileNetV3 search space per OFA \cite{ofa}.

\subsection{Dataset generalization}
We use a batch size of 128 for all \proposedTraining and BigNAS experiments. We empirically find SGD to be superior to RMSProp and report all BigNAS results on CIFAR-10, CIFAR-100 and ImageNet-100 with SGD. On all 3 datasets, teacher model for OFA is trained using SGD with CosineAnnealingLR. After teacher training, we train OFA for a total of 250 epochs split as depth phase 1 (25 epochs), depth phase 2 (120 epochs), expand phase 1 (25 epochs) and expand phase 2 (120 epochs) with the learning rates and schedules for each phase per \ofaCite. 

\subsubsection{CIFAR-10/CIFAR-100}

We train \proposedTraining for 200 epochs, with an initial learning rate of 0.1. We regularize \proposedTraining with a weight decay of 5e-4 and dropout of 0.1. We use a full model warmup period of 100 epochs (\fullModelWarmupSym=50\%) for \proposedTraining. We train BigNAS with an initial learning rate of 0.1 and a constant ending at 5\% of the initial lr. We use the same number of epochs and regularization as \proposedTraining. 

\subsubsection{ImageNet-100}
The ImageNet-100 dataset is a subset of the ImageNet-1k dataset created by \cite{imagenet100}. \proposedTraining is trained for 180 epochs, with an initial learning rate of 0.143, weight decay of 5e-4, and dropout 0.1. We use a full warmup period of 100 epochs (\fullModelWarmupSym=55\%). BigNAS is trained with the same hyperparameters as \proposedTraining with changes such as learning rate decay with constant ending, regularizing only the largest network and initialization of batch norm layers.

% \section{Appendix D: }

\bibliographystyle{plain}
\bibliography{bibs/related_work, bibs/misc, bibs/datasets}
